# Supplementary material for: Dissecting the Interplay of Attention Paths in a Statistical Mechanics Theory of Transformers
Source: arXiv:2405.15926 source file (2024-12-08)
Supplement: Supplementary file 1 [file supmat_old.tex]

\appendix

\section{Derivation of the kernel renormalization theory}
\subsection{Model definition}
\label{app:model_definition}
We remind the definition of our transformer model from Sec.~\ref{sec:Model} of the main text. We first expand the bare input $x^{\left(0\right)}\in\mathbb{R}^{N_{0}\times{T}}$ to $x^{\left(1\right)}\in\mathbb{R}^{N_{1}\times{T}}$ by a linear transformation: $x_{i,t}^{\left(1\right)}=\frac{1}{\sqrt{N_{0}}}\sum_{j=1}^{N_{0}}V_{ij}^{\left(0\right)}x_{j,t}^{\left(0\right)}$, where $V^{(0)}_{ij}$ are learnable parameters, $i=1,\ldots,N_{1}$, and  $t=1,\ldots,T$. We can then define the output from each attention layer $ \ell=1,\ldots,L$ recursively:
\begin{equation}
x_{i,t}^{\left(\ell+1\right)}=\frac{1}{\sqrt{N_{\ell}{H}_{\ell}}}\sum_{s=1}^{{T}}\sum_{h=1}^{{H}_{\ell}}\sum_{j=1}^{N_{\ell}}V_{ij}^{\left(\ell\right)h}x_{j,s}^{\left(\ell\right)}\Omega_{st}^{\left(\ell\right)h}\qquad i=1,\ldots,N_{\ell+1}\;,\qquad t=1,\ldots,T\;,
\end{equation}
where $H_\ell$ and $N_\ell$ denote respectively the number of heads and the width of the $\ell$-th layer, while for simplicity in the main text we set $N_\ell=N$, $H_\ell=H$ for each $\ell$. The attention matrix $\Omega^{\left(\ell\right)h}\in\mathbb{R}^{T\times T}$ is defined
as
\begin{equation}
\Omega_{st}^{\left(\ell\right)h}=\zeta\left(\frac{\beta}{N_{0}\sqrt{G}}x_{s}^{\left(0\right)\top}\cdot K^{\left(\ell\right)h}\cdot Q^{\left(\ell\right)h}\cdot x_{t}^{\left(0\right)}\right)\;.
\end{equation}
The function $\zeta$ denotes the softmax applied along the direction of the $s$-th token, while the hyperparameter $\beta$ controls the ``hardness'' of the softmax function. The readout is linear and is parametrized by $a\in\mathbb{R}^{1\times N_{L+1}}$
\begin{equation}
    f=\frac{1}{\sqrt{N_{L+1}}}a\cdot x_{i,t^{*}}^{\left(L+1\right)}\;,
\end{equation}
where we adopt the unified notation
\begin{equation}
    \;\;x_{i,t^{*}}^{\left(L+1\right)}=\begin{cases}
        \frac{1}{T}\sum_{t=1}^Tx_{i,t}^{\left(L+1\right)}&\qquad \text{average over all the tokens}\\\\
\;\;x_{i,1}^{\left(L+1\right)}&\qquad\text{reading from the first token}
\\\\
\;\;x_{i,T}^{\left(L+1\right)}&\qquad\text{reading from the last token}
    \end{cases}\;\;,
\end{equation}
in order to consider different types of tasks. 
\paragraph{Effective description ---} 
It is useful to collect the value matrices into a set of ``effective weights''
\begin{equation}
V^{\left(\mathrm{eff}\right)h_{1}h_{2}\ldots h_{L}}\coloneqq a\cdot V^{\left(L\right)h_{L}}\cdot V^{\left(L-1\right)h_{L-1}}\cdot\ldots\cdot V^{\left(2\right)h_{2}}\cdot V^{\left(1\right)h_{1}}\;.
\end{equation}
We also define the ``attentioned input'' 
\begin{equation}
\xi^{(0)h_{1}h_{2}\ldots h_{L}}\coloneqq\sum_{t_{0},\ldots,t_{L-1}=1}^{T}x_{t_{0}}^{\left(0\right)}\Omega_{t_{0}t_{1}}^{\left(1\right)h_{1}}\Omega_{t_{1}t_{2}}^{\left(2\right)h_{2}}\ldots\Omega_{t_{L-2}t_{L-1}}^{\left(L-1\right)h_{L-1}}\Omega_{t_{L-1}t^{*}}^{\left(L\right)h_{L}}\;.
\end{equation}
In what follows, it is useful to introduce a compact notation for the ``effective input'' to each layer
\begin{equation}
    \xi^{\left(L-\ell\right)h_{L-\ell}\ldots h_{L}}\coloneqq\frac{1}{\sqrt{N_{L-\ell-1}H_{L-\ell-1}}}\sum_{t_{L-\ell}, \ldots,t_{L-1}=1}^Tx_{t_{L-\ell}}^{\left(L-\ell\right)}\Omega_{t_{L-\ell}t_{L-\ell+1}}^{\left(L-\ell\right)h_{L-\ell}}\ldots\Omega_{t_{L-1},t^*}^{\left(L\right)h_{L}}\;,
\end{equation}
$\ell=1,\ldots,L-1$, and for the last attention layer
\begin{equation}
    \xi^{\left(L\right)h_L}\coloneqq\frac{1}{\sqrt{N_{L-1} H_{L-1}}}\sum_{h_{L-1}=1}^{H_{L-1}} V^{(L-1)h_{L-1}}\xi^{(L-1)h_{L-1}h_L}\;.
\end{equation}

\begin{figure}
    \centering
    \hspace{-1em}\includegraphics[width=1.1\textwidth]{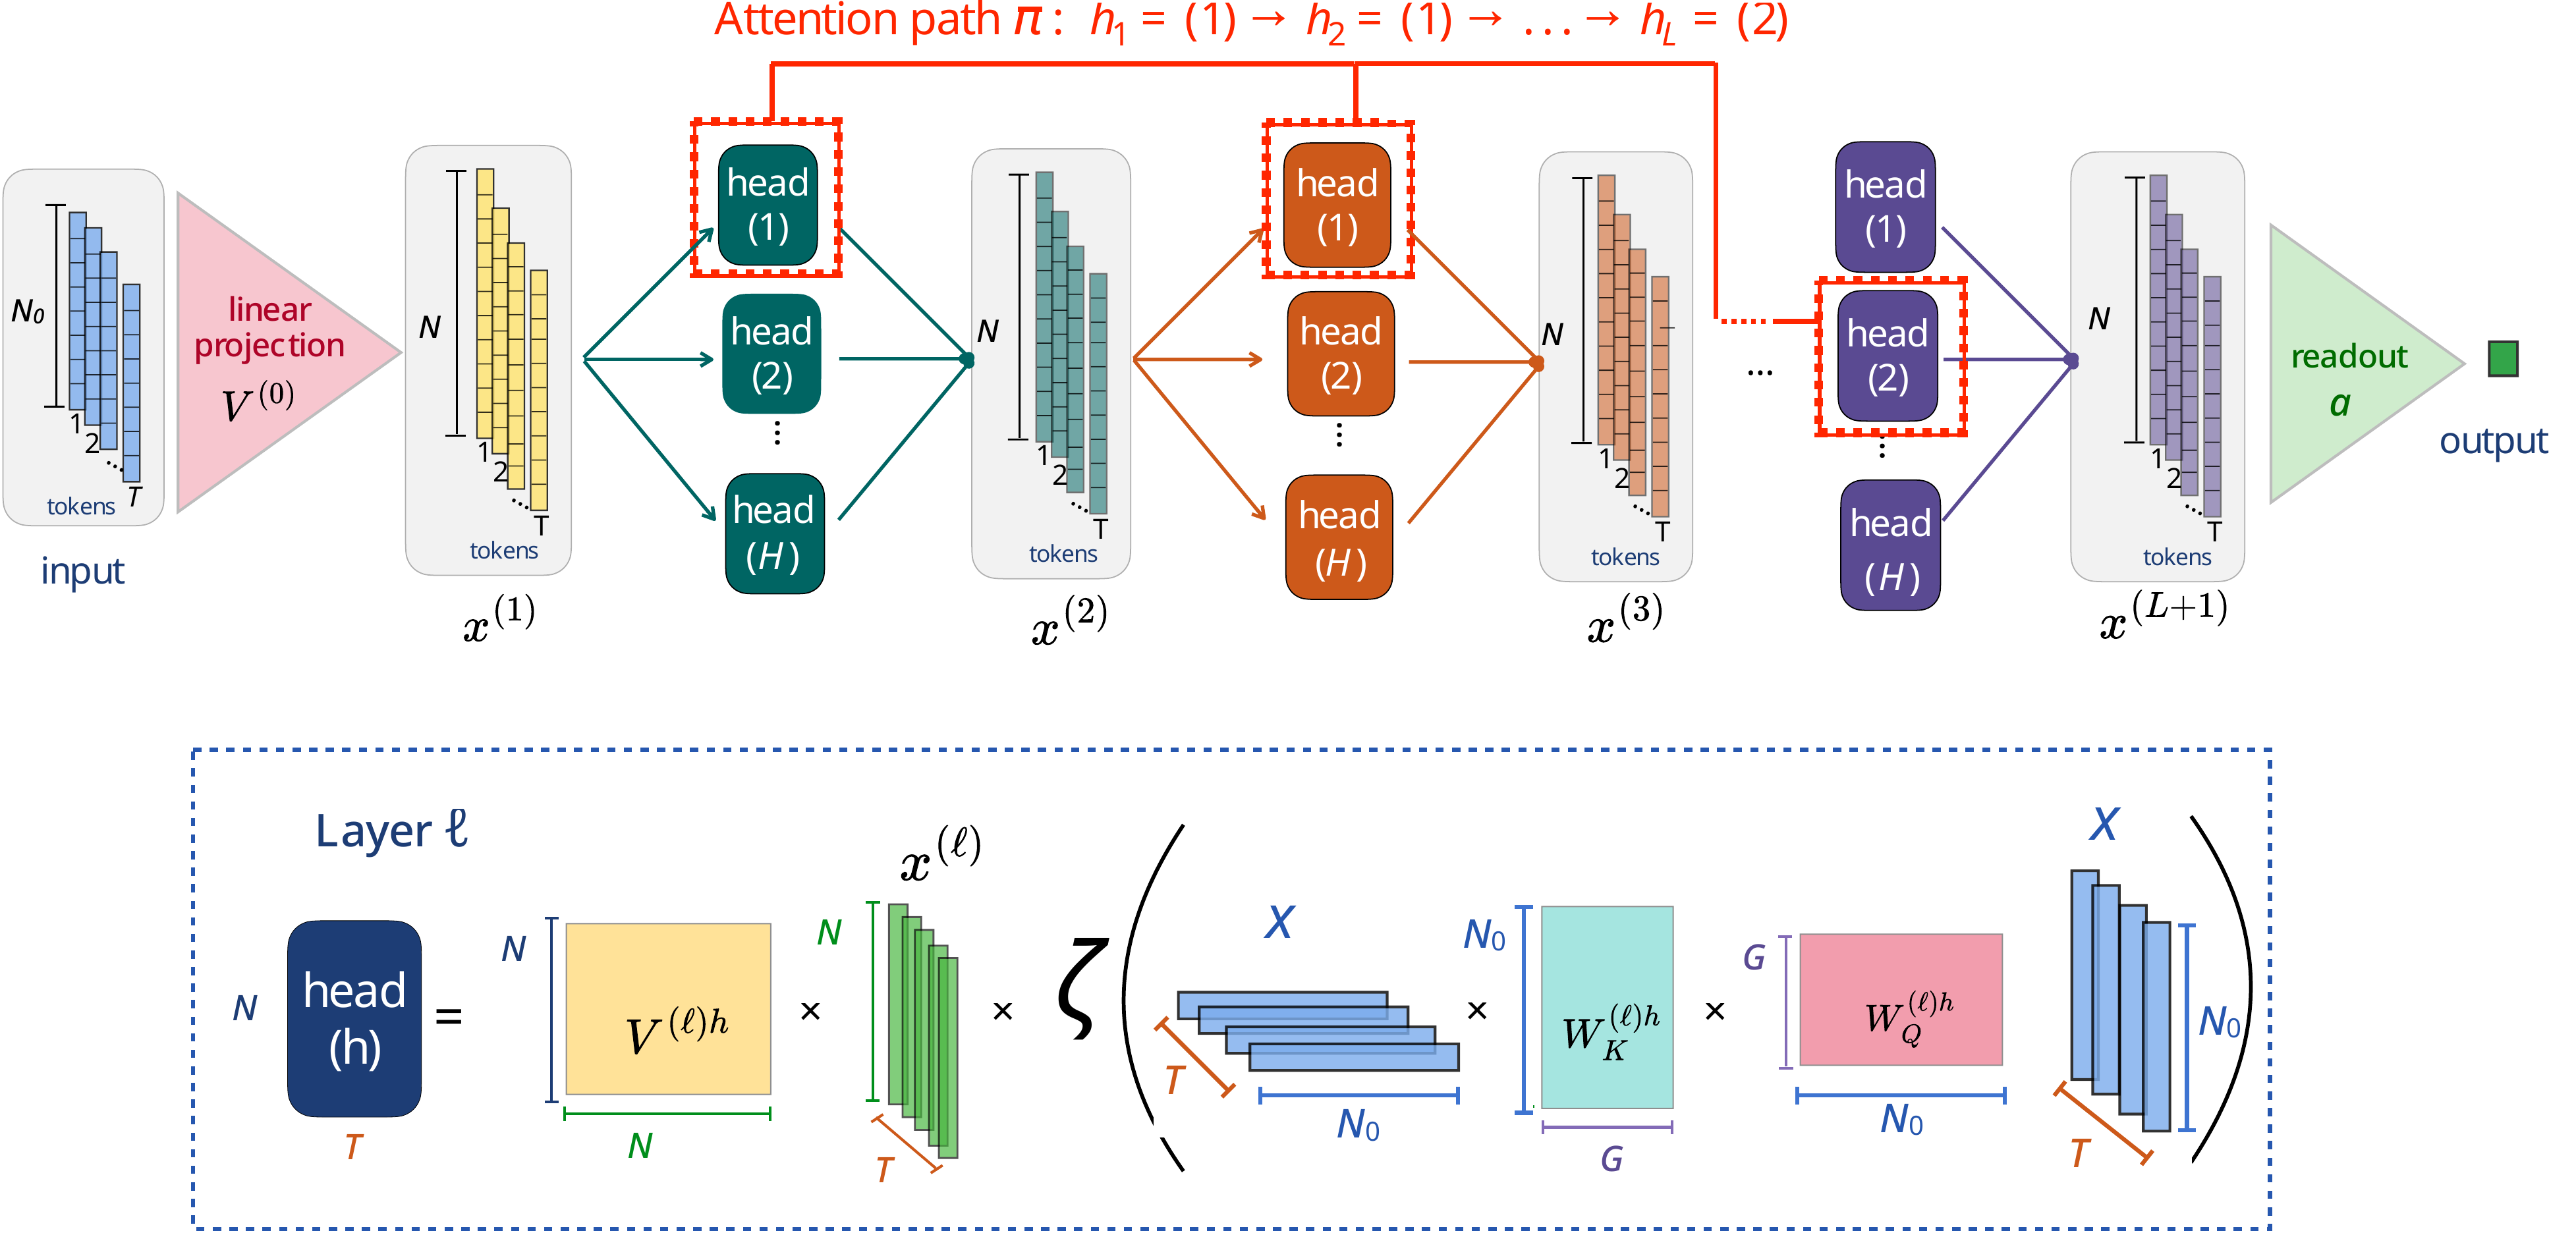}
    \caption{Schematic representation of the architecture under consideration.}
    \label{fig:illustration}
\end{figure}

\subsection{Posterior distribution}
We are interested in computing the posterior distribution over the network's learnable weights $\Theta\coloneqq\left(V^{\left(0\right)},\left\{ V^{\left(\ell\right)h}\right\} _{\ell,h=1}^{L,H},a\right)$. This is analogous to the Gibbs distribution in statistical physics and is defined as
\begin{equation}
p\left(\Theta\right)=\frac 1 Z \exp\left\{ -\frac{1}{2\mathcal{T}}\sum_{\mu=1}^{P}\left[f\left(x^{\left(0\right)\mu},\Theta\right)-y^{\mu}\right]^{2}-\frac{1}{2\sigma^{2}}\left\Vert \Theta\right\Vert ^{2}\right\} \;,
\end{equation}
where $Z$ indicates the normalization, also called partition function, and $\mathcal{T}$ is the Gibbs temperature. \Fnotes{def Frobenius norm in general} It is useful to introduce a set of auxiliary variables $\{\tt^\mu\}_{\mu=1}^P$ in order to linearize the squared error. The partition function then reads
\begin{align}
   Z\propto \int \dd\Theta\,\dd\tt \,\exp\left(-\frac{\mathcal{T}}{2}\Vert\tt\Vert^2 -\frac{1}{2\sigma^2}\Vert \Theta\Vert^2 +\sum_{\mu=1}^P\ii \tt^\mu\left(f\left(x^{\left(0\right)\mu},\Theta\right)-y^{\mu}\right)\right)\;,
\end{align}
where we have used the symbol $``\propto"$ to indicate that we are neglecting multiplicative constants. We can progressively integrate over all the learnable weights, starting from the readout $a$ and proceeding backwards through the value weights $V^{(\ell)h}$ until the first projection layer $V^{(0)}$. This procedure follows the lines of \citep{li2021statistical,li2022globally}.
\paragraph{Integral over the readout weights ---} We start by computing the integral over the readout weights $a\in\mathbb{R}^{N_{L+1}}$:
\begin{equation}
\begin{split}
    Z\propto\\\int \dd V^{(0)}\left[\prod_{\ell=1}^L\prod_{h_\ell=1}^{H_\ell}\dd V^{(\ell)h_\ell}\right]\dd \tt\exp\left(-\frac{\mathcal{T}}{2}\Vert\tt\Vert^2-\frac{1}{2\sigma^2}\Vert V^{(0)}\Vert^2 -\frac{1}{2\sigma^2}\sum_{\ell=1}^L\sum_{h_\ell=1}^{H_\ell}\Vert V^{(\ell)h_\ell}\Vert^2 \right)\\\times\int \dd a \exp\left(-\frac{1}{2\sigma^2}\Vert a\Vert^2-\sum_{\mu=1}^P\ii \tt^\mu y^\mu +\sum_{\mu=1}^P\ii \tt^\mu\frac{a^\top x_{t^*}^{(L+1),\mu}}{\sqrt{N_{L+1}}}\right)\\
    \propto\int \dd V^{(0)}\left[\prod_{\ell=1}^L\prod_{h_\ell=1}^{H_\ell}\dd V^{(\ell)h_\ell}\right]\dd \tt\exp\left(-\frac{1}{2\sigma^2}\Vert V^{(0)}\Vert^2 -\frac{1}{2\sigma^2}\sum_{\ell=1}^L\sum_{h=1}^{H_\ell}\Vert V^{(\ell)h_\ell}\Vert^2 \right)\\\times
    \exp\left(-\sum_{\mu=1}^P\ii \tt^\mu y^\mu-\frac{\mathcal{T}}{2}\Vert\tt\Vert^2-\frac{\sigma^2}{2 }\sum_{\mu,\nu=1}^P\tt^\mu \tt^\nu\frac{{x_{t^*}^{(L+1),\mu}}^\top x_{t^*}^{(L+1),\nu}}{N_{L+1}} \right)\;.
\end{split}
\end{equation}
\Fnotes{Here I do not think we need to keep track of all multiplicative constants as for the physical interpretation}
Moreover, given that we are interested in the minima of the loss landscape, we can set the Gibbs temperature to zero $\mathcal{T}=0$.
\paragraph{Integral over the value weights at layer $L$ ---} We continue our backward integration starting from the last value weights $V^{(L)}$:
\begin{equation}
\begin{split}
    Z\propto \int \dd V^{(0)}\left[\prod_{\ell=1}^{L-1}\prod_{h_\ell=1}^{H_\ell}\dd V^{(\ell)h_\ell}\right]\dd \tt \exp\left(-\frac{1}{2\sigma^2}\Vert V^{(0)}\Vert^2 -\frac{1}{2\sigma^2}\sum_{\ell=1}^{L-1}\sum_{h_\ell=1}^{H_\ell}\Vert V^{(\ell)h_\ell}\Vert^2 \right)\\\times\exp\left(-\sum_{\mu=1}^P\ii \tt^\mu y^\mu\right)\\\times \int \left[\prod_{h=1}^{H_L}\dd V^{(L)h}\right]\exp\left(-\frac{1}{2\sigma^2}\sum_{h_\ell=1}^{H_L}\Vert V^{(L)h_\ell}\Vert^2\right)\\\times\exp\left(-\frac{\sigma^2}{2}\sum_{\mu,\nu=1}^P \tt^\mu \tt^\nu\frac{\sum_{h_L,\tilde h_L=1}^{H_L}{\xi^{(L)h_L,\mu}}^\top {V^{(L)h_L}}^\top V^{(L)\tilde h_L}\xi^{(L)\tilde h_L, \nu}}{N_{L+1} N_L H_L}\right)\;.
    \end{split}
\end{equation}
The first index in $V^{(L)h_L}$ can be factored out, which leaves us with $N_{L+1}$ identical copies of the integral
\begin{equation}
\begin{split}
    \int\left[ \prod_{h_L=1}^{H_L}\prod_{j=1}^{N_L}\dd V^{(L)h_L}_{1j}\right]\exp\left(-\frac 12 \sum_{h_L,\tilde h_L=1}^{H_L}\sum_{i,j=1}^{N_L}V^{(L)h_L}_{1i}\left[\frac{\delta_{ij}\delta_{h_L \tilde h_L}}{\sigma^2}+v_i^{h_L}v_j^{\tilde h_L}\right]V_{1j}^{(L)\tilde h_L}\right)\\\propto
    \frac{1}{\sqrt{\det\left(\text{Id}+\sigma^2 vv^\top\right)}}
    \end{split}
\end{equation}
\Fnotes{Here I use the most simplified notation where again all constants go in the $``\propto''$}
where we define
\begin{equation}
    v_i^{h_L}\coloneqq\sqrt{\frac{\sigma^4}{N_{L+1}N_LH_L}}\sum_{\mu=1}^P\tt^\mu \xi_i^{(L)h_L,\mu}\;,
\end{equation}
and we denote by $v$ the vector whose indices run over the pair $(i,h_L)$. Applying the matrix determinant lemma: $\det\left(\text{Id}+\sigma^2 vv^\top\right)=1+\sigma^2 v^\top v$, we find
\begin{equation}
\begin{split}
    Z\propto\int \dd V^{(0)}\left[\prod_{\ell=1}^{L-1}\prod_{h_\ell=1}^{H_\ell}\dd V^{(\ell)h_\ell}\right]\dd \tt \exp\left(-\frac{1}{2\sigma^2}\Vert V^{(0)}\Vert^2 -\frac{1}{2\sigma^2}\sum_{\ell=1}^{L-1}\sum_{h_\ell=1}^{H_\ell}\Vert V^{(\ell)h_\ell}\Vert^2 \right)\\\times\exp\left(-\sum_{\mu=1}^P\ii \tt^\mu y^\mu-\frac{N_{L+1}}{2}\log\left(1+\frac{\sigma^2}{N_{L+1}}\sum_{\mu,\nu=1}^P\tt^\mu \tt^\nu C^{(L+1),\mu\nu}\right)\right)\;,
\end{split}
\end{equation}
where we have defined the \emph{pre-kernel} $C^{(L+1),\mu\nu}$ as
\begin{equation}
    C^{(L+1),\mu\nu}\coloneqq \frac{\sigma^2}{N_L H_L}\sum_{h_L=1}^{H_L}{\xi^{(L)h_L,\mu}}^\top \xi^{(L)h_L,\nu}\;.
\end{equation}
\paragraph{Order parameter at layer $L$ ---} We introduce the definition of the following order parameter
\begin{equation}
    H^{(L+1)}\coloneqq \frac{\sigma^2}{N_{L+1}}\sum_{\mu,\nu=1}^P\tt^\mu \tt^\nu C^{(L+1),\mu\nu}\;,
\end{equation}
and its Fourier conjugate $U^{(L+1)}$. The partition function can be written as 
\begin{equation}
\begin{split}
 Z   \propto \int \dd H^{(L+1)}\,\dd U^{(L+1)}\,\dd \tt\, \dd V^{(0)}\exp\left(-\sum_{\mu=1}^P\ii \tt^\mu y^\mu+\frac{N_{L+1}}{2\sigma^2}H^{(L+1)} U^{(L+1)}\right)\\\times\exp\left(-\frac{N_{L+1}}{2}\log\left(1+H^{(L+1)}\right)-\frac{1}{2\sigma^2}\Vert V^{(0)}\Vert^2\right)\\\times\int \left[\prod_{\ell=1}^{L-1}\prod_{h_\ell=1}^{H_\ell}\dd V^{(\ell)h_\ell}\right]\exp\left(-\frac{1}{2\sigma^2}\sum_{\ell=1}^{L-1}\sum_{h_\ell=1}^{H_\ell}\Vert V^{(\ell)h_\ell}\Vert^2-\frac{1}2 U^{L+1}\sum_{\mu,\nu}\tt^\mu \tt^\nu C^{(L+1),\mu\nu}\right)\;.
 \end{split}
\end{equation}
\paragraph{Integral over the value weights at layer $(L-1)$ ---}


\section{Physical interpretation of the order parameter}
\begin{figure}[ht!]
    \centering
    \includegraphics[width=1\textwidth]{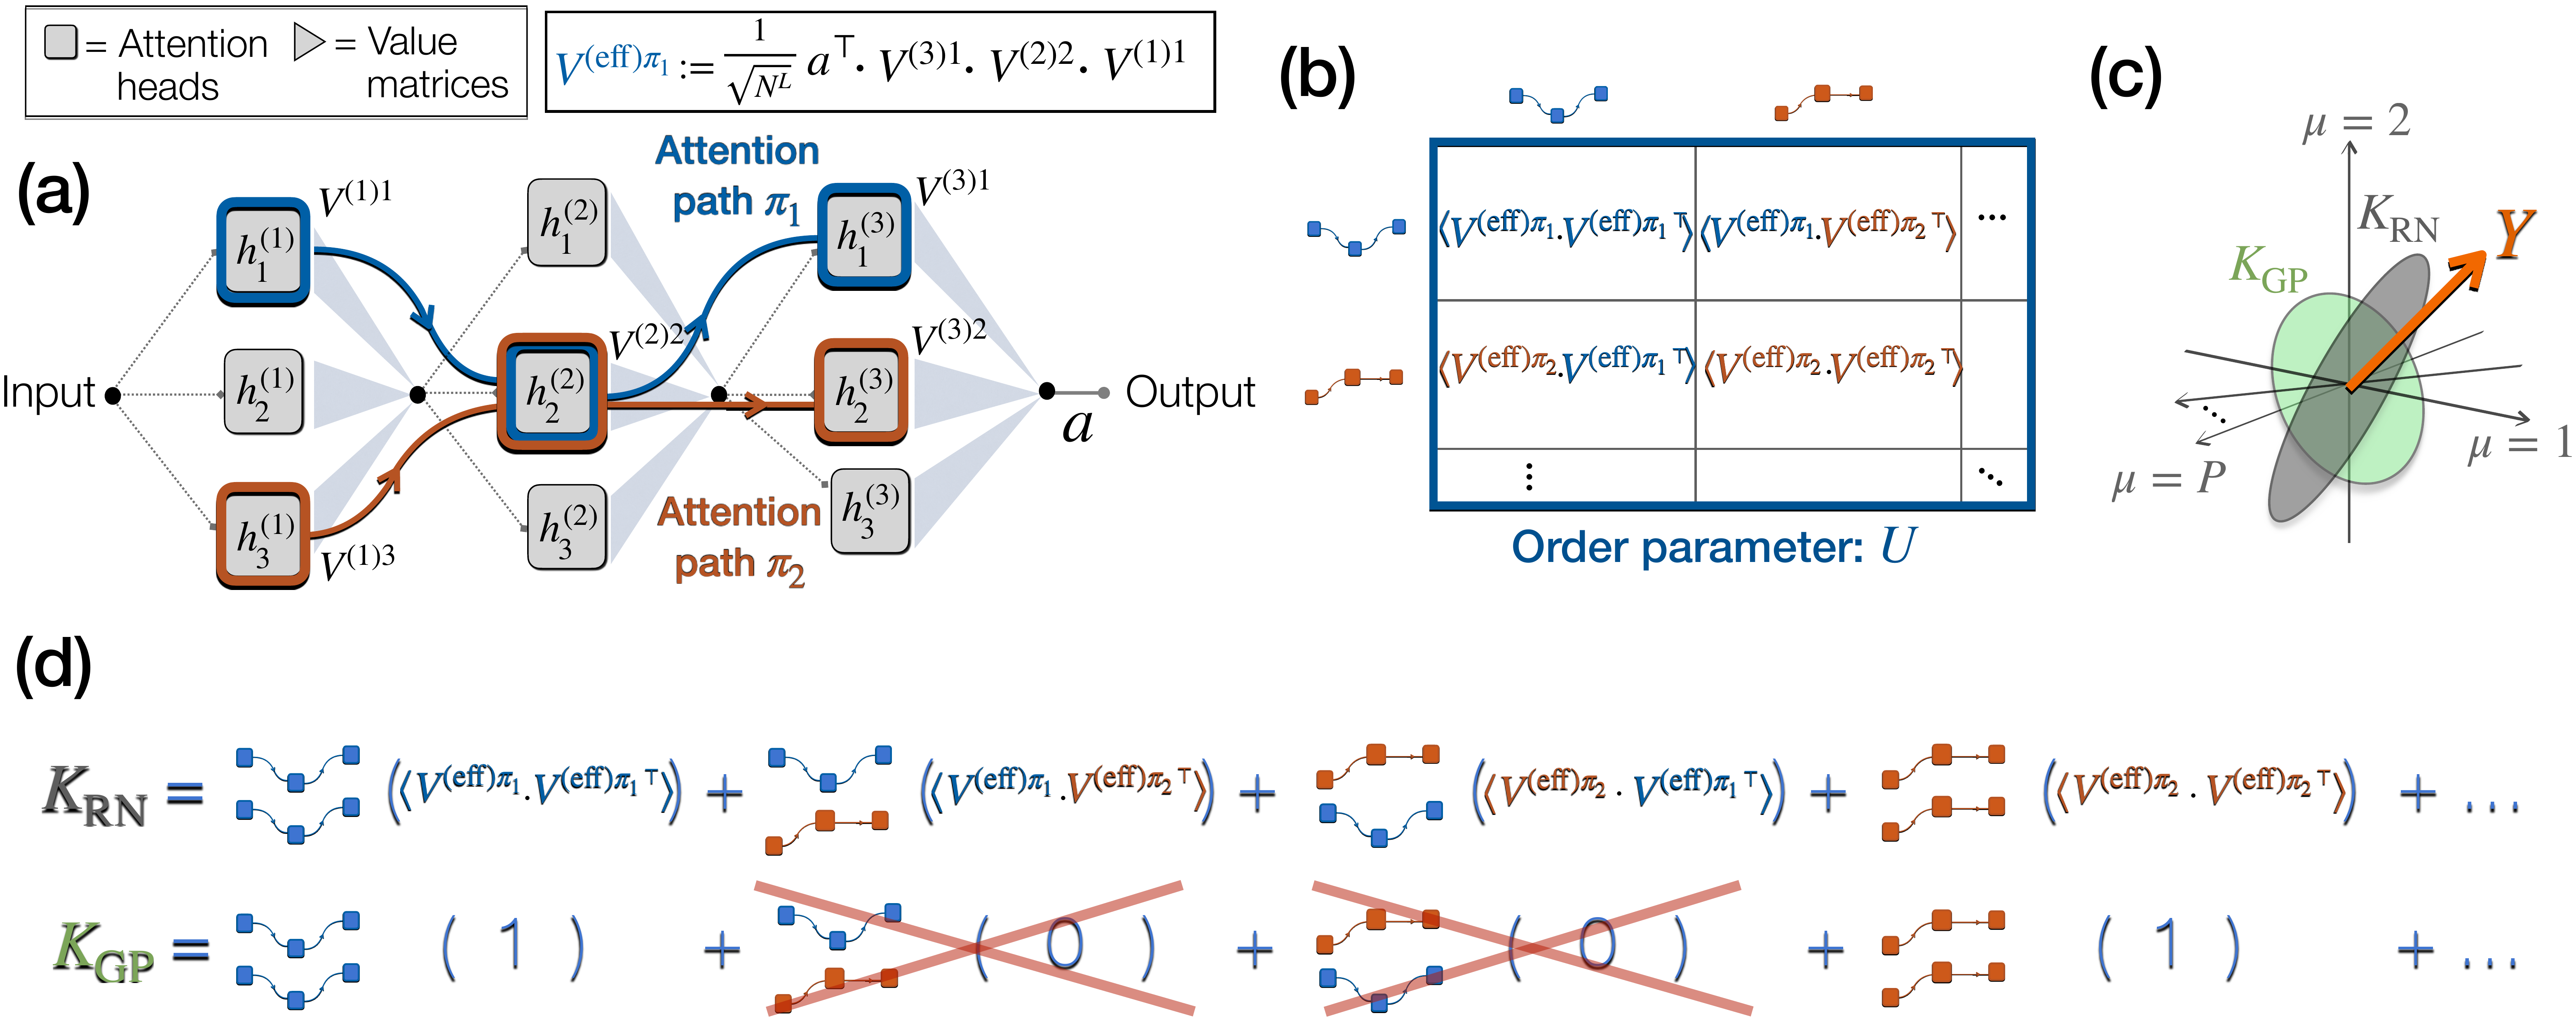}
    \caption{Caption}
    \label{fig:enter-label}
\end{figure}
